# Supplementary material for: Instruction-Guided Autoregressive Neural Network Parameter Generation
Source: arXiv:2504.02012 source file (2025-04-02)
Supplement: Supplementary file 1 [file appendix.tex]

\newpage
\appendix
\onecolumn
\section{Additional Details}\label{app:sec1}
\subsection{Weights Vectorization}
For a neural network with $L$ layers, the process of vectorizing the weights and biases for both fully connected and convolutional layers is as follows:\
\begin{itemize}
    \item For the l\textsuperscript{th} fully connected layer: 
  $W^{(l)} \in \mathbb{R}^{d_{l-1} \times d_l} \rightarrow \text{vec}(W^{(l)}) \in \mathbb{R}^{d_{l-1}.d_l}$ and $b^{(l)} \in \mathbb{R}^{d_l}$. The length of the vectorized weights for this layer, including the bias if it is not null, is given by \( d_{l-1}d_l + d_l \).
  \item For the l\textsuperscript{th} convolutional layer: 
  $W^{(l)} \in \mathbb{R}^{k_h . k_w.c_{in}.c_{out}}$ and $b^{(l)} \in \mathbb{R}^{c_{out}}$. The length of the vectorized weights for this layer, including the bias if it is not null, is \( k_h \cdot k_w \cdot c_{in} \cdot c_{out} + c_{out} \).
\end{itemize}
We then concatenate all the flattened weight and bias vectors  resulting in vector $\theta$: $ \theta = \bigoplus_{l=1}^{L} \left( \text{vec}(W^{(l)}) \oplus b^{(l)} \right)$\
Where $\text{vec}$ denotes the vectorization operation and $\oplus$ denotes concatenation. 
This compactly represents vectorizing and concatenating weights and biases for any layer type. The concatenation keeps the ordering of weights in the network.

\subsection{Weights Vectors Chunking}
The chunking mechanisms briefly discuss in the methods section is broken down as follows. Let the pretrained weights of the network be denoted by a tensor \( W \in \mathbb{R}^{d_1 \times d_2 \times \dots \times d_n} \) which are then flattened into a vector \( w \in \mathbb{R}^{D} \), where \( D = d_1 \times d_2 \times \dots \times d_n \). Chunking the weight vector assume the flattened vector \( w \) is divided into \( N \) chunks, each of size \( C \), such that \( D = N \times C \). Let the chunks be represented as \( w_i \in \mathbb{R}^{C} \) for \( i = 1, 2, \dots, N \).

\textbf{VAE Chunks Encoding: }As described in the approach section, each chunk \( w_i \) is encoded using a Variational Autoencoder (VAE). The encoder of the VAE maps \( w_i \) to a latent representation \( z_i \) such that:     $z_i = f_{\text{VAE-enc}}(w_i) \in \mathbb{R}^{L}$, where \( f_{\text{VAE-enc}} \) is the encoding function and \( L \) is the dimensionality of the latent space. The latent representations \( z_1, z_2, \dots, z_N \) are concatenated to form a single vector: $ z_{\text{concat}} = [z_1, z_2, \dots, z_N] \in \mathbb{R}^{N \times L}$
    
\textbf{VQ-VAE Encoding}: The concatenated latent vector \( z_{\text{concat}} \) is then encoded using a Vector Quantized VAE (VQ-VAE) whose encoder maps \( z_{\text{concat}} \) to a discrete latent code \( z_q \) from a finite codebook: $ z_q = f_{\text{VQ-VAE-enc}}(z_{\text{concat}}) \in \text{Codebook}$. The discrete code is decoded back to a latent space \( \hat{z}_{\text{concat}} \) using the VQ-VAE decoder:    $\hat{z}_{\text{concat}} = f_{\text{VQ-VAE-dec}}(z_q)$

\textbf{Reconstructing of the Weights}: The reconstructed latent vector \( \hat{z}_{\text{concat}} \) is split back into \( N \) latent vectors: $\hat{z}_i \in \mathbb{R}^{L} \quad \text{for } i = 1, 2, \dots, N$ where each \( \hat{z}_i \) is passed through the VAE decoder to reconstruct the original chunks:    $\hat{w}_i = f_{\text{VAE-dec}}(\hat{z}_i) \in \mathbb{R}^{C}$. Finally, the chunks \( \hat{w}_i \) are concatenated to form the reconstructed weight vector: $\hat{w} = [\hat{w}_1, \hat{w}_2, \dots, \hat{w}_N] \in \mathbb{R}^{D}$.
To enable sampling The transformer  prior is applied to the generated codebook of concatenated chunks.
The spatial order and consistency in sampling are measured by the performance of the sampled weights compared to the original weights.

% 2. **Sampling from VQ-VAE:**
%    - Sampling from the VQ-VAE means selecting a code \( q \) from the codebook, which corresponds to a latent vector \( \hat{z}_{\text{concat}} \).
%    - Since \( \hat{z}_{\text{concat}} \) is constructed to represent the concatenated latent space \( z_{\text{concat}} \), which in turn was derived from spatially ordered chunks of the original weights, the decoding of this sampled latent vector should yield spatially consistent reconstructions.
%    - This spatial consistency is preserved if the VQ-VAE is trained such that the codebook entries (and hence the sampled latent codes) correspond to meaningful and consistent regions in the latent space.

% 3. **No Loss in Spatial Information:**
%    - Since \( \hat{w}_i = w_i \) for all \( i \), the spatial information inherent in the original weight vector \( w \) is preserved in the reconstruction \( \hat{w} \).
%    - Even when sampling, the structure and ordering of the chunks in the latent space ensure that the reconstructed weights maintain the spatial relationship present in the original network's weights.

% Thus, the VQ-VAE sampling does not lose any spatial information of the full vectorized weights as long as the reconstruction is perfect and the latent space preserves the spatial consistency.

\subsection{Architectures} We use a modified version of the VAE used in Latent diffusion by inserting a linear layer as the first input layer and another as output layer to adapt the vectorized weights such that we can properly reshape them for convolution layer input. In the training process, we remove the discrimintor loss as well as the LiPs loss. We made similar settings for VQGAN by removing the perpexity loss, and kept the min-gpt exactly the same except the input dimmension.

\textbf{Task descriptions}: For the image datasets used in our experiments, we selected 5 images per class to construct the conditioning data. These samples were randomly selected during training to allow the model to map a large number of data points to the pre-trained weights. In the case of NLP tasks, we generated fixed descriptions for each task without providing any examples from the tasks themselves.
%%%%%%%%%%%%%%%%%%%%%%%
\begin{itemize}
    \item  \textbf{sts-b: } \textit{Your task is to predict the similarity score between two sentences. These scores indicate how similar the sentences are in terms of meaning. Please rate their similarity on a scale from 0 to 5, where 0 indicates no meaning overlap, 1 indicates very little overlap, and 5 indicates complete overlap in meaning.}
    \item \textbf{mrcp: } \textit{Your task is to determine the semantic equivalence of two given sentences, referred to as Sentence 1 and Sentence 2. If the sentences are semantically equivalent, return 1. If they are not, return 0.}
    \item  \textbf{sst2: }\textit{Your task is to determine the sentiment of a given sentence. Respond with 0 if the sentiment is negative and 1 if the sentiment is positive}
    \item  \textbf{cola: }\textit{Your task is to evaluate whether the given sentence is both syntactically and semantically correct. If it is, respond with "1"; otherwise, respond with "0"}
    \item  \textbf{Qnli: } \textit{Your task is to evaluate whether the given response properly answers the provided question. If the response answers the question correctly, return 0; otherwise, return 1}
    \item  \textbf{Rte: }\textit{Your task is to determine if a given hypothesis is true (entailment), false (contradiction), or undetermined (neutral) based on a provided premise.}
\end{itemize}

%%%%%%%%%%%%%%%%%%%%%

\subsection{Pretrained Zoos}
\textbf{Modelzoo dataset}: The datasets used for the experiments in Table \ref{tab:hyperzoo} were drawn from the collection of pretrained models provided by~\cite{schurholt2022model}. Specifically, for the MNIST and SVHN datasets, we utilized their small CNN model, which comprises three convolutional layers and two fully connected layers, totaling 2,464 parameters. For the STL10 and CIFAR-10 datasets, we employed their large CNN model, consisting of 10,853 parameters. We then combined the weights from each respective models(\{MNIST+SVHN\} and \{CIFAR-10, STL-10\}), resulting in a total of $\approx 6000$ training for each model. For each architecture and dataset, we utilize pre-trained weights from epochs 21 to 25, resulting in a total of 5,000 samples per dataset. The data is split into 70\% for training, 15\% for testing, and 15\% for validation.

\textbf{Glue Experiments}: For the GLUE experiments, we followed the same setup as \cite{gao2024parameterefficientfinetuningdiscretefourier} to generate the model zoo by saving the last 10 epochs, resulting in 60 pretrained weight vectors with a maximum length of 616132 parameters. We applied the same approach to the ViT LoRA model, as these tasks are classification-based.

\textbf{Gumbel Softmax}: Here we provide detailed information about equation \ref{eqn:gqant2} presented in the method section.
\begin{equation}
    z_q = \sum_{j=1}^{K} y_j \mathbf{e}_j
    ,\label{eqn:gqant2}
\end{equation}
% \[
% \y_i = \frac{\exp\left((\log \pi_i + g_i)/\tau\right)}{\sum_{j=1}^{k} \exp\left((\log \pi_j + g_j)/\tau\right)}
% \]
where $y_j$ is the gumbel softmax output of the latent representation: $y_j = \frac{\exp\left((\log \pi_j + g_j) / \tau\right)}{\sum_{i=1}^{K} \exp\left((\log \pi_i + g_i) / \tau\right)}$  
where:
- \(\log \pi_i\) are the logits from the model.
- \(g_i \sim \text{Gumbel}(0,1)\) are i.i.d. samples.
- \(\tau > 0\) is a temperature parameter that controls the smoothness of the distribution. As \(\tau \rightarrow 0\), \(y_j\) approaches a one-hot vector, making the sample more discrete.

\section{Additional Experiments}

\subsection{Additional Results with LoRA} 
We expanded the performance evaluation by applying LoRA to vision-based image classification tasks, as shown in Table \ref{tab:cv}. The results demonstrate that our method effectively learns the distribution of LoRA weights, optimized across diverse image datasets, and the associated classification heads, all within a single generative model. 
\input{AnonymousSubmission/LaTeX/tables/lora-vit}
As demonstrated in Table \ref{tab:cv}, by merely learning the conditional distribution of the pretrained models, we achieve an improvement in performance exceeding 10\%. The maximum weight vector length is 222725.

\subsection{Additional experiment on convergence speed}
In this experiment we investigated whether simply using a conditional VAE would have led to similar performance as \ourmethod. In this experiments we used combined zoos of all dataaset with minimum weights vector length 2464 and maximum 2864.
We observed that fine-tuning weights with higher initial accuracy on MNIST and SVHN datasets resulted in lower final performance compared to those with lower initial accuracy. Consequently, we report only the configurations that ensure rapid convergence, specifically by changing the temperature and top-k parameters of \ourmethod to enable generating weights with low initial performance for SVHN an MNIST that can boost the fine-tuning. Although HyperCVAE struggled to perform well at initialization across various settings, HyperVQGAN demonstrated stronger initial performance, achieving average accuracies of 82.15±0.32 on MNIST and 66.35±5.14 on SVHN. The top-k sampling strategy employed by HyperVQGAN facilitates the generation of diverse weights, enhancing its robust performance and providing greater flexibility in exploring the weight space.
The convergence evolution is reported in Figure \ref{neuripsevol} and the performance at initial state, first  epoch and last epochs are reported in Table \ref{sample-table}
\input{tables/table1}

\begin{figure}[t!]
    \centering
    % \vspace{-0.1in}
     \begin{subfigure}{0.24\linewidth}
            \includegraphics[width=1.0\textwidth]{img/indist_plot_mnist_fig.pdf}
            \caption{MNIST}
            \label{figmnist}
    \end{subfigure}
    % \vspace{-0.1in}
     \begin{subfigure}{0.24\linewidth}
            \includegraphics[width=1.0\textwidth]{img/indist_plot_svhn_fig.pdf}
            \caption{SVHN}
            \label{figsvhn}
    \end{subfigure}
    % \vspace{-0.1in}
     \begin{subfigure}{0.24\linewidth}
            \includegraphics[width= 1.0\textwidth]{img/indist_plot_cifar-10_fig.pdf}
            \caption{CIFAR-10}
            \label{figcifar}
    \end{subfigure}
    % \vspace{-0.1in}
     \begin{subfigure}{0.24\linewidth}
	\includegraphics[width=1.0\textwidth]{img/indist_plot_stl-10_fig.pdf}
        \caption{STL-10}
         \label{figstl}
    \end{subfigure}
	% \vspace{-0.13in}
        \caption{Average accuracy progression during fine-tuning over 25 epochs with sampled weights. The sampled weights are evaluated on the same pre-trained datasets to compare their performance against both the existing method and the original pre-trained model.}
        \label{neuripsevol}
	% \vspace{-0.15in}
\end{figure}

\subsection{Tas-adaptive sampling for unseen dataset}
We evaluate \ourmethod on a cross-dataset adaptation task by first learning the distribution of combined pretrained models trained on MNIST and CIFAR-10, and then evaluating the performance on SVHN and STL-10 datasets, as well as the inverse scenario. The experiment leverages the small zoo introduced in \cite{schurholt2022model}, with 2,864 parameters allocated for STL-10 and CIFAR-10, and 2,464 parameters for MNIST and SVHN.

\begin{figure}[t!]
    \centering
    \vspace{-0.1in}
     \begin{subfigure}{0.24\linewidth}
            \includegraphics[width=1.0\textwidth]{img/cross_plot_mnist_fig.pdf}
            \caption{MNIST}
            \label{figmnist}
    \end{subfigure}
    % \vspace{-0.1in}
     \begin{subfigure}{0.24\linewidth}
            \includegraphics[width=1.0\textwidth]{img/cross_plot_svhn_fig.pdf}
            \caption{SVHN}
            \label{figsvhn}
    \end{subfigure}
    % \vspace{-0.1in}
     \begin{subfigure}{0.24\linewidth}
            \includegraphics[width= 1.0\textwidth]{img/cross_plot_cifar-10_fig.pdf}
            \caption{CIFAR-10}
            \label{figcifar}
    \end{subfigure}
    % \vspace{-0.1in}
     \begin{subfigure}{0.24\linewidth}
	\includegraphics[width=1.0\textwidth]{img/cross_plot_stl-10_fig.pdf}
        \caption{STL-10}
         \label{figstl}
    \end{subfigure}
	% \vspace{-0.13in}
        \caption{The assessment of cross-dataset transfer learning begins by initializing the model with sampled weights, which is then fine-tuned over 25 epochs. The model's performance is evaluated against three benchmarks: the baseline model, a model trained from scratch with random weight initialization, and pretrained models.}
        \label{fig:cross}
	\vspace{-0.15in}
\end{figure}

\subsection{Effect of Fine-Tuning Sampled Weights on Domain Generalization} 
In this section, we investigate the impact of sampled weights based fine-tuning on generalization compared to the pretrained weights based fine-tuning.
The experiments are conducted based on unconditional HyperVQGAN with  chunk-based encoding with chunk size 49152.
\par \textbf{Generalization test on OfficeHome dataset} is carried out following the training procedure of DIWA \cite{rame2022diwa}. We learned the distribution of the Resnet50 pretrained feature extractor then sampled weights to initialize Resnet50 for the DiWA method. We also do the same experiment using the pretrained weights-based initialization. 
\par The results show in Table \ref{tab344} that DIWA with our initialization outperforms the original work on 3 out of 4 classification tasks with average accuracy 73.63$\pm$0.18\% versus 72.80\% for the baseline DIWA. This experiment showed that the proposed method sampling-based initialization generalizes well across tasks. 
\input{tables/table6}
%---------------------------------------------------------------
\section{Robustness Against Adversarial Attacks Compare to the Pretrained Model.}
\textbf{Task:} We investigate whether our HyperVQGAN sampling approach results in vulnerability to adversarial attack compared to the pretrained weights. We use Lenet-5\cite{Haykin2001GradientBasedLA} for this experiment. The model is trained on each of the 4 MNIST datasets as shown in Table \ref{tab4w}. 
\par \textbf{Results:} We sampled one sample of architecture weights per datasets and compared the results to the top-1 accuracy as shown in Table \ref{tab4w}.

\begin{table}[h!]
\caption{Top 1 pretrained accuracy versus one sample of sampling using HyperVQGAN}
\label{tab4w}
% \vskip 0.15in
\begin{center}
\begin{small}
\begin{sc}
\resizebox{0.8\columnwidth}{!}{% <------ Don't forget this %
\begin{tabular}{lccccr}
\hline
Model & \#params. & code vec. & pretrained & sampled \\
\hline
MNIST & 2572& 36& 98.363& 98.363\\
Fashion-MNIST &2572&36& 89.57& 89.570\\
kMNIST& 2572&36& 91.52& 91.52\\
EMNIST & 2572& 36& 88.611 & 88.59\\
\hline
\end{tabular}
}
\end{sc}
\end{small}
\end{center}
\vskip -0.1in
\end{table}

We then perform successive adversarial attacks using the same set of sampled weights, comparing the model's performance to that of the pretrained model. The results, detailed in Tables \ref{tab5w}, illustrate the adversarial robustness of the models under Fast Gradient Sign Method (FGSM) ~\cite{Madry2017TowardsDL} and Projected Gradient Descent (PGD) ~\cite{Goodfellow2014ExplainingAH} attacks. Our experiments reveal that the model based on sampled weights not only maintains but often surpasses the adversarial robustness of the pretrained model. These findings indicate that the proposed sampling technique preserves, and can even enhance, the adversarial robustness of pretrained models. 

\begin{table}[h!]
\begin{center}
 \begin{subtable}[h]{0.8\columnwidth}
\caption{Fast Gradient Sign Attack(FGSM).}
\label{tab5w}
% \vskip 0.15in
\begin{center}
\begin{small}
\begin{sc}
% \resizebox{0.\columnwidth}{!}{% <------ Don't forget this %
\begin{tabular}{lcccr}
\hline
Model & epsilon & pretrained & sampled \\
\hline
MNIST & 0.007& 97.97& 97.97\\
Fashion-MNIST &0.007& 87.21& 87.22\\
kMNIST& 0.007& 89.63&89.64\\
EMNIST & 0.007&  86.62 &86.65\\
\hline
MNIST & 0.05& 94.78& 94.79\\
Fashion-MNIST &0.05& 69.25& 69.25\\
kMNIST& 0.05& 75.28&75.32\\
EMNIST & 0.05&  72.92 &72.92\\
\hline
\end{tabular}
% }
\end{sc}
\end{small}

\end{center}
\vskip -0.1in
\end{subtable}
 \begin{subtable}[h]{0.49\columnwidth}
\caption{Projected gradient descent(PGD) attack.}
\label{tab6}
% \vskip 0.15in
\begin{center}
\begin{small}
\begin{sc}
% \resizebox{0.49\columnwidth}{!}{% <------ Don't forget this %
\begin{tabular}{lcccr}
\hline
Model & epsilon & pretrained & sampled \\
\hline
MNIST & 8/255& 95.19& 95.19\\
Fashion-MNIST &8/255& 66.24& 66.25\\
kMNIST& 8/255& 75.69&75.70\\
EMNIST & 8/255&  66.62 &66.65\\
\hline
MNIST & 16/255& 90.85& 90.85\\
Fashion-MNIST &16/255& 43.51& 43.51\\
kMNIST& 16/255& 58.13&58.04\\
EMNIST & 16/255&  41.87 &41.85\\
\hline
\end{tabular}
% }
\end{sc}
\end{small}
\end{center}
\vskip -0.1in
\end{subtable}
     \caption{results of robustness to adversarial attacks}
     \label{tabb}
\end{center}
\end{table}

\subsection{Pretrained Weights Retrival Through Sampling} 
One application of our method is in weights retrieval for transfer learning. HyperVQGAN can conditionally learn the distribution of multiple pretrained models, enabling dataset-specific weight retrieval. To demonstrate this capability, we divided Tiny-ImageNet into 20 non-overlapping datasets, each containing 10 classes. We then trained a LeNet model on each dataset for 50 epochs across 5 runs. After training, we collected the final epoch checkpoints and jointly learned the distribution of the pretrained weights.\\ 
\textbf{Results}: The results of this experiment are reported in Table \ref{tab35e}
In this experiment we prove that our approach can learn the distribution of many checkpoints from diverse datasets as shown in Table\ref{tab35e}. The results are based on Lenet5, and our chunk-free approach is used with GPT sampler. This can allow in practice to get access to multiple pretrained weights from diverse tasks for fine-tuning, or transfer learning. 
 % \begin{table}[t]
\begin{table}[h]
\vskip -0.15in
 % \begin{flushright}
 \caption{Weights retrieval through sampling from pretrained distribution. Average accuracy of 5 pretrained models and 5 samples of sampling for each subset dataset on Tiny-ImageNet with no extra training.}
\label{tab35e}
\vskip -0.15in
\begin{center}
\begin{small}
\begin{sc}
\resizebox{0.49\columnwidth}{!}{% <------ Don't forget this %
\begin{tabular}{lccr}
\hline
 Dataset& Pretrained & sampled&  \\
\hline
subset\_0 & 49.36$\pm$1.03 & \textbf{49.60 $\pm$1.31}\\
subset\_1 & \textbf{43.56$\pm$1.47} & 43.55 $\pm$1.52\\
subset\_2 & 53.16$\pm$1.02 & \textbf{53.40$\pm$3.04}\\
subset\_3 & \textbf{46.16$\pm$1.64} & 46.04$\pm$1.62\\
subset\_4 & \textbf{43.40$\pm$0.1.13} & 43.27 $\pm$1.29\\
\hline
subset\_5 & 47.61$\pm$1.93 & \textbf{47.73 $\pm$1.70}\\
subset\_6 & \textbf{46.524$\pm$2.43} & 46.36 $\pm$2.64\\
subset\_7 & 46.04$\pm$0.44 & \textbf{46.60$\pm$0.44}\\
subset\_8 & 40.32$\pm$2.81 & \textbf{40.64$\pm$2.61}\\
subset\_9 & \textbf{50.48$\pm$2.80} & 50.40 $\pm$2.86\\
\hline
subset\_10 & \textbf{48.83$\pm$1.34} & 48.76 $\pm$1.05\\
subset\_11 & 49.63$\pm$1.20 & \textbf{49.64 $\pm$0.86}\\
subset\_12 & \textbf{33.32$\pm$1.13} & 33.16$\pm$1.23\\
subset\_13 & 46.84$\pm$1.60 & \textbf{46.92$\pm$1.44}\\
subset\_14 & \textbf{36.88$\pm$1.27} & 36.88 $\pm$1.10\\
\hline
subset\_15 & \textbf{50.08$\pm$1.97} & 49.96 $\pm$1.92\\
subset\_16 & 48.36$\pm$0.85 & \textbf{48.52 $\pm$0.82}\\
subset\_17 & 44.08$\pm$2.83 & \textbf{44.16$\pm$2.76}\\
subset\_18 & \textbf{49.00$\pm$2.00} & 48.96$\pm$2.10\\
subset\_19 & 40.52$\pm$0.1.31 & \textbf{40.68$\pm$1.10}\\
\hline
\end{tabular}
}
\end{sc}
\end{small}
\end{center}
\vskip -0.1in
\end{table}
% \end{table}
